# Supplementary material for: Breaking Boundaries: Balancing Performance and Robustness in Deep Wireless Traffic Forecasting
Source: arXiv:2311.09790 source file (2023-11-28)
Supplement: Supplementary file 1 [file files.tex]

\begin{table*}[htb]
\caption{Information about the original balanced datasets \ro{Should we keep this one? Very large}}
\label{info_data}
\begin{center}
{\footnotesize
\begin{tabular}{lccccccccc}
\toprule
Dataset & n\_classes & Train\_size & Dim & Length & Var\_train & Var\_test & Im\_ratio & d\_train\_test & prop\_miss \\
\midrule
Adiac                          &        37 &           390 &         1 &    176 &           0.12 &          0.12 &    18.14 &         0.14 &              0 \\
CBF                            &         3 &            30 &         1 &    128 &           0.24 &          0.17 &     0.13 &         1.87 &              0 \\
Car                            &         4 &            60 &         1 &    577 &           0.21 &          0.23 &     0.15 &         1.61 &              0 \\
CharacterTrajectories          &        20 &   e       1422 &         3 &    182 &           0.15 &          0.15 &    13.06 &         3.35 &           0.33 \\
ChlorineConcentration          &         3 &           467 &         1 &    166 &           0.22 &          0.21 &     1.25 &         0.26 &              0 \\
CinCECGTorso                   &         4 &            40 &         1 &   1639 &            0.2 &          0.13 &     0.31 &         4.81 &              0 \\
CricketX                       &        12 &           390 &         1 &    300 &           0.16 &          0.15 &     5.08 &         0.46 &              0 \\
CricketY                       &        12 &           390 &         1 &    300 &           0.15 &          0.15 &     6.04 &         0.55 &              0 \\
CricketZ                       &        12 &           390 &         1 &    300 &           0.15 &          0.16 &     6.07 &         0.38 &              0 \\
DistalPhalanxOutlineAgeGroup   &         3 &           400 &         1 &     80 &           0.18 &           0.2 &     1.41 &         0.87 &              0 \\
DistalPhalanxOutlineCorrect    &         2 &           600 &         1 &     80 &           0.12 &          0.15 &     0.17 &         0.85 &              0 \\
DistalPhalanxTW                &         6 &           400 &         1 &     80 &           0.18 &          0.21 &     3.47 &         0.68 &              0 \\
DodgerLoopDay                  &         7 &            78 &         1 &    288 &            0.2 &          0.21 &     3.04 &        16.33 &           0.01 \\
ECG200                         &         2 &           100 &         1 &     96 &           0.21 &           0.2 &     0.25 &         0.77 &              0 \\
ECG5000                        &         5 &           500 &         1 &    140 &           0.14 &          0.09 &     2.73 &         0.34 &              0 \\
ECGFiveDays                    &         2 &            23 &         1 &    136 &           0.23 &          0.16 &     0.14 &         2.06 &              0 \\
EOGHorizontalSignal            &        12 &           362 &         1 &   1250 &           0.13 &          0.11 &     9.01 &       586.54 &              0 \\
EOGVerticalSignal              &        12 &           362 &         1 &   1250 &           0.11 &          0.11 &     9.01 &      2228.29 &              0 \\
Earthquakes                    &         2 &           322 &         1 &    512 &           0.19 &          0.22 &     0.45 &         2.34 &              0 \\
EigenWorms                     &         5 &           128 &         6 &  17984 &           0.18 &          0.18 &     3.26 &       386.95 &              0 \\
ElectricDevices                &         7 &          8926 &         1 &     96 &           0.07 &          0.07 &     3.31 &         0.72 &              0 \\
Epilepsy                       &         4 &           137 &         3 &    206 &           0.18 &          0.18 &     1.05 &         6.03 &              0 \\
EthanolConcentration           &         4 &           261 &         3 &   1751 &           0.24 &          0.23 &        2 &       101616 &              0 \\
FaceFour                       &         4 &            24 &         1 &    350 &           0.26 &          0.21 &     1.24 &         4.46 &              0 \\
FacesUCR                       &        14 &           200 &         1 &    131 &           0.16 &          0.13 &     9.25 &         0.68 &              0 \\
FingerMovements                &         2 &           316 &        28 &     50 &           0.16 &          0.18 &        0 &       588.92 &              0 \\
Fish                           &         7 &           175 &         1 &    463 &           0.17 &          0.17 &     1.08 &         0.83 &              0 \\
FordA                          &         2 &          3601 &         1 &    500 &           0.14 &          0.16 &     0.02 &         0.81 &              0 \\
FordB                          &         2 &          3636 &         1 &    500 &           0.14 &          0.16 &     0.02 &         0.92 &              0 \\
GesturePebbleZ1                &         6 &           132 &         1 &    455 &            0.2 &          0.15 &     1.05 &        93.94 &           0.49 \\
GesturePebbleZ2                &         6 &           146 &         1 &    455 &            0.2 &          0.15 &     3.02 &       108.44 &           0.51 \\
GunPoint                       &         2 &            50 &         1 &    150 &           0.25 &          0.22 &     0.03 &         1.05 &              0 \\
GunPointAgeSpan                &         2 &           135 &         1 &    150 &           0.32 &           0.3 &        0 &       239.69 &              0 \\
GunPointMaleVersusFemale       &         2 &           135 &         1 &    150 &           0.32 &           0.3 &     0.03 &       248.23 &              0 \\
GunPointOldVersusYoung         &         2 &           136 &         1 &    150 &           0.32 &           0.3 &     0.03 &       183.39 &              0 \\
Ham                            &         2 &           109 &         1 &    431 &           0.17 &          0.18 &     0.03 &         2.73 &              0 \\
HandOutlines                   &         2 &          1000 &         1 &   2709 &            0.1 &          0.12 &     0.18 &         2.18 &              0 \\
Handwriting                    &        26 &           150 &         3 &    152 &           0.15 &           0.1 &    12.23 &         4.04 &              0 \\
Haptics                        &         5 &           155 &         1 &   1092 &           0.18 &          0.16 &     0.24 &         1.47 &              0 \\
Heartbeat                      &         2 &           204 &        61 &    405 &           0.09 &          0.09 &      0.3 &        23.15 &              0 \\
Herring                        &         2 &            64 &         1 &    512 &            0.2 &          0.22 &     0.14 &         1.06 &              0 \\
InlineSkate                    &         7 &           100 &         1 &   1882 &            0.2 &          0.16 &     3.13 &         4.37 &              0 \\
InsectEPGRegularTrain          &         3 &            62 &         1 &    601 &           0.41 &          0.39 &     0.34 &         0.09 &              0 \\
InsectEPGSmallTrain            &         3 &            17 &         1 &    601 &           0.42 &          0.39 &     0.31 &         0.37 &              0 \\
ItalyPowerDemand               &         2 &            67 &         1 &     24 &           0.22 &          0.16 &     0.01 &         0.18 &              0 \\
LSST                           &        14 &          2459 &         6 &     36 &           0.03 &          0.02 &     9.49 &      2259.42 &              0 \\
Lightning2                     &         2 &            60 &         1 &    637 &           0.19 &          0.19 &     0.22 &         4.46 &              0 \\
Lightning7                     &         7 &            70 &         1 &    319 &           0.19 &          0.19 &     3.22 &         1.98 &              0 \\
Mallat                         &         8 &            55 &         1 &   1024 &           0.22 &          0.17 &     3.24 &          1.4 &              0 \\
MedicalImages                  &        10 &           381 &         1 &     99 &           0.14 &          0.13 &      7.5 &         0.46 &              0 \\
MelbournePedestrian            &        10 &          1194 &         1 &     24 &           0.16 &          0.14 &     1.01 &        50.98 &              0 \\
MiddlePhalanxOutlineAgeGroup   &         3 &           400 &         1 &     80 &           0.16 &          0.19 &     1.31 &         1.06 &              0 \\
MiddlePhalanxOutlineCorrect    &         2 &           600 &         1 &     80 &           0.14 &          0.16 &     0.19 &         0.88 &              0 \\
MiddlePhalanxTW                &         6 &           399 &         1 &     80 &           0.17 &          0.22 &     3.34 &         0.36 &              0 \\
NonInvasiveFetalECGThorax1     &        42 &          1800 &         1 &    750 &            0.1 &          0.12 &    21.06 &         0.31 &              0 \\
NonInvasiveFetalECGThorax2     &        42 &          1800 &         1 &    750 &           0.09 &          0.11 &    21.06 &         0.21 &              0 \\

\multicolumn{10}{r}{\footnotesize(Continued next page)}
\bottomrule
\end{tabular}
} % font size
\end{center}
\end{table*}

\begin{table*}[htb]
\label{fig:info_data}
\begin{center}
{\footnotesize
\begin{tabular}{lccccccccc}
\toprule
Dataset & n\_classes & Train\_size & Dim & Length & Var\_train & Var\_test & Im\_ratio & d\_train\_test & prop\_miss \\
\midrule
OSULeaf                        &         6 &           200 &         1 &    427 &            0.2 &           0.2 &     2.21 &         1.47 &              0 \\
OliveOil                       &         4 &            30 &         1 &    570 &           0.23 &          0.22 &     1.29 &         0.03 &              0 \\
PEMS-SF                        &         7 &           267 &       963 &    144 &           0.17 &          0.18 &     3.07 &        30.79 &              0 \\
PLAID                          &        11 &           537 &         1 &   1344 &           0.13 &          0.12 &     4.38 &       216.46 &           0.76 \\
PenDigits                      &        10 &          7494 &         2 &      8 &            0.3 &          0.29 &     4.02 &        12.53 &              0 \\
PhalangesOutlinesCorrect       &         2 &          1800 &         1 &     80 &           0.09 &          0.12 &      0.2 &         0.52 &              0 \\
Plane                          &         7 &           105 &         1 &    144 &           0.22 &          0.23 &     2.15 &         1.18 &              0 \\
ProximalPhalanxOutlineAgeGroup &         3 &           400 &         1 &     80 &            0.2 &          0.23 &      0.3 &          0.1 &              0 \\
ProximalPhalanxOutlineCorrect  &         2 &           600 &         1 &     80 &           0.17 &          0.21 &     0.24 &         0.11 &              0 \\
ProximalPhalanxTW              &         6 &           400 &         1 &     80 &            0.2 &          0.21 &     3.47 &         0.15 &              0 \\
RacketSports                   &         4 &           151 &         6 &     30 &           0.14 &          0.14 &     1.06 &        19.56 &              0 \\
SelfRegulationSCP1             &         2 &           268 &         6 &    896 &           0.16 &          0.15 &        0 &      3352.33 &              0 \\
SonyAIBORobotSurface1          &         2 &            20 &         1 &     70 &           0.25 &          0.16 &     0.27 &         1.12 &              0 \\
SonyAIBORobotSurface2          &         2 &            27 &         1 &     65 &           0.25 &          0.15 &     0.12 &         0.86 &              0 \\
SpokenArabicDigits             &        10 &          6599 &        13 &     93 &           0.14 &          0.13 &        0 &        38.48 &           0.57 \\
StarLightCurves                &         3 &          1000 &         1 &   1024 &           0.17 &          0.13 &     1.29 &         0.41 &              0 \\
Strawberry                     &         2 &           613 &         1 &    235 &           0.15 &          0.15 &     0.19 &         0.37 &              0 \\
SwedishLeaf                    &        15 &           500 &         1 &    128 &           0.14 &          0.14 &     7.07 &         0.27 &              0 \\
Symbols                        &         6 &            25 &         1 &    398 &           0.27 &          0.22 &     3.21 &         2.93 &              0 \\
Trace                          &         4 &           100 &         1 &    275 &           0.26 &          0.26 &      1.1 &         2.05 &              0 \\
TwoLeadECG                     &         2 &            23 &         1 &     82 &           0.27 &          0.16 &     0.03 &         0.63 &              0 \\
TwoPatterns                    &         4 &          1000 &         1 &    128 &           0.26 &          0.26 &     1.03 &         0.42 &              0 \\
UWaveGestureLibraryAll         &         8 &           896 &         1 &    945 &           0.18 &          0.16 &     4.04 &         1.19 &              0 \\
UWaveGestureLibraryX           &         8 &           896 &         1 &    315 &           0.17 &          0.16 &     4.04 &          0.9 &              0 \\
UWaveGestureLibraryY           &         8 &           896 &         1 &    315 &           0.19 &          0.17 &     4.04 &         0.53 &              0 \\
UWaveGestureLibraryZ           &         8 &           896 &         1 &    315 &           0.18 &          0.16 &     4.04 &         0.56 &              0 \\
Wafer                          &         2 &          1000 &         1 &    152 &           0.26 &          0.23 &     0.61 &         0.74 &              0 \\
Wine                           &         2 &            57 &         1 &    234 &           0.22 &          0.25 &     0.03 &         0.15 &              0 \\
WordSynonyms                   &        25 &           267 &         1 &    270 &           0.18 &          0.17 &    18.39 &         0.94 &              0 \\
Worms                          &         5 &           181 &         1 &    900 &            0.2 &          0.22 &     3.25 &         3.32 &              0 \\
WormsTwoClass                  &         2 &           181 &         1 &    900 &            0.2 &          0.22 &     0.11 &         3.32 &              0 \\
Yoga                           &         2 &           300 &         1 &    426 &           0.22 &          0.21 &     0.06 &         1.15 &              0 \\

\bottomrule
\end{tabular}
} % font size
\end{center}

\end{table*}

\begin{table*}[htb]

\caption{Accuracy for ROCKET baseline model on balanced datasets of the UCR/UEA archive \tr{add 5 scatter plots graph with a diagonal line (everything above diagonal means that augmentation wins)} \ro{scatter plot added in the main content of the paper, now maybe we can remove this one?}}
\label{rocket_results}
\begin{center}
{\footnotesize
\begin{tabular}{lcccccc}
\toprule
Dataset &  rocket &  rocket\_noise\_1.0 &  rocket\_noise\_3.0 &  rocket\_noise\_5.0 &  rocket\_smote &  rocket\_timegan \\
\midrule
Adiac                          &   78.52 &             73.35 &             72.58 &             72.99 &         79.80 &           80.77 \\
CBF                            &  100.00 &             99.78 &             99.73 &             99.89 &         99.87 &           99.89 \\
Car                            &   90.67 &             92.00 &             93.33 &             93.00 &         89.67 &           91.67 \\
CharacterTrajectories          &   98.52 &             99.09 &             99.04 &             99.12 &         98.47 &           99.19 \\
ChlorineConcentration          &   81.77 &             73.70 &             72.07 &             71.70 &         82.49 &           74.61 \\
CinCECGTorso                   &   83.74 &             81.26 &             80.96 &             81.07 &         86.59 &           82.71 \\
CricketX                       &   81.79 &             81.69 &             81.44 &             80.72 &         82.62 &           81.28 \\
CricketY                       &   85.23 &             84.41 &             84.56 &             84.82 &         85.49 &           84.36 \\
CricketZ                       &   85.74 &             84.31 &             83.54 &             83.54 &         84.92 &           84.87 \\
DistalPhalanxOutlineAgeGroup   &   75.54 &             74.53 &             73.96 &             75.25 &         70.22 &           74.82 \\
DistalPhalanxOutlineCorrect    &   77.10 &             76.59 &             76.45 &             76.38 &         77.54 &           77.46 \\
DistalPhalanxTW                &   72.09 &             67.63 &             66.47 &             66.91 &         64.60 &           72.09 \\
DodgerLoopDay                  &   56.75 &             59.75 &             60.00 &             58.00 &         60.00 &           60.50 \\
ECG200                         &   90.00 &             92.40 &             91.80 &             92.00 &         91.60 &           88.40 \\
ECG5000                        &   94.73 &             94.30 &             94.10 &             94.20 &         94.51 &           94.48 \\
ECGFiveDays                    &  100.00 &            100.00 &            100.00 &            100.00 &        100.00 &          100.00 \\
EOGHorizontalSignal            &   63.76 &             63.70 &             63.43 &             63.26 &         64.25 &           63.54 \\
EOGVerticalSignal              &   54.25 &             53.81 &             54.53 &             54.92 &         53.70 &           54.48 \\
Earthquakes                    &   74.82 &             74.24 &             74.82 &             74.82 &         74.53 &           74.82 \\
EigenWorms                     &   89.16 &             79.54 &             82.60 &             83.97 &         91.15 &           88.93 \\
ElectricDevices                &   72.81 &             71.47 &             72.26 &             72.70 &         72.71 &           72.92 \\
Epilepsy                       &   98.99 &             98.12 &             98.41 &             98.26 &         98.55 &           99.28 \\
EthanolConcentration           &   41.29 &             39.16 &             40.08 &             40.53 &         42.43 &           42.05 \\
FaceFour                       &   97.50 &             96.59 &             97.27 &             97.73 &         97.73 &           97.73 \\
FacesUCR                       &   96.17 &             95.84 &             95.28 &             95.29 &         96.39 &           95.47 \\
FingerMovements                &   52.20 &             54.80 &             54.00 &             55.00 &         53.80 &           54.80 \\
Fish                           &   98.17 &             97.71 &             96.80 &             97.49 &         98.29 &           97.94 \\
FordA                          &   94.52 &             94.32 &             94.29 &             94.41 &         94.29 &           94.30 \\
FordB                          &   80.40 &             80.62 &             80.05 &             80.59 &         80.42 &           80.52 \\
GesturePebbleZ1                &   43.49 &             43.72 &             47.56 &             48.14 &         43.02 &           54.65 \\
GesturePebbleZ2                &   20.38 &             33.42 &             32.91 &             33.67 &         20.51 &           31.01 \\
GunPoint                       &  100.00 &             99.33 &             99.33 &             99.33 &        100.00 &          100.00 \\
GunPointAgeSpan                &   99.68 &             99.62 &             99.62 &             99.62 &         99.68 &           99.68 \\
GunPointMaleVersusFemale       &   99.75 &             99.68 &             99.68 &             99.68 &         99.87 &           99.68 \\
GunPointOldVersusYoung         &   99.17 &             98.98 &             99.05 &             99.11 &         98.98 &           99.05 \\
Ham                            &   71.62 &             72.76 &             72.19 &             72.57 &         71.81 &           72.76 \\
HandOutlines                   &   94.27 &             93.51 &             93.41 &             93.73 &         94.70 &           93.46 \\
Handwriting                    &   58.71 &             59.13 &             56.61 &             56.78 &         59.91 &           57.93 \\
Haptics                        &   52.14 &             50.91 &             50.97 &             50.84 &         53.05 &           51.69 \\
Heartbeat                      &   73.76 &             73.07 &             74.63 &             72.59 &         75.32 &           74.34 \\
Herring                        &   70.00 &             71.56 &             70.94 &             69.69 &         58.13 &           65.00 \\
InlineSkate                    &   46.15 &             44.04 &             44.18 &             44.22 &         47.38 &           44.18 \\
InsectEPGRegularTrain          &  100.00 &             99.20 &             98.47 &             98.80 &         99.68 &           99.28 \\
InsectEPGSmallTrain            &   98.23 &             96.47 &             95.58 &             95.02 &         97.51 &           95.98 \\
ItalyPowerDemand               &   96.93 &             96.97 &             97.08 &             97.10 &         96.91 &           96.93 \\
LSST                           &   63.84 &             61.97 &             62.54 &             62.64 &         61.39 &           63.78 \\
Lightning2                     &   75.74 &             77.05 &             76.72 &             76.07 &         80.66 &           74.43 \\
Lightning7                     &   82.19 &             80.00 &             77.81 &             82.47 &         83.01 &           81.92 \\
Mallat                         &   95.58 &             95.82 &             95.91 &             95.97 &         95.33 &           96.21 \\
MedicalImages                  &   79.92 &             77.29 &             73.47 &             74.34 &         76.47 &           76.50 \\
MelbournePedestrian            &   90.48 &             90.41 &             90.29 &             90.45 &         90.73 &           90.52 \\
MiddlePhalanxOutlineAgeGroup   &   59.22 &             64.42 &             62.99 &             63.12 &         51.69 &           57.79 \\
MiddlePhalanxOutlineCorrect    &   83.71 &             83.99 &             83.85 &             84.26 &         81.44 &           83.30 \\
MiddlePhalanxTW                &   55.45 &             59.87 &             60.65 &             56.49 &         52.73 &           54.42 \\
NonInvasiveFetalECGThorax1     &   95.51 &             92.65 &             92.32 &             92.37 &         95.63 &           95.04 \\
NonInvasiveFetalECGThorax2     &   96.85 &             95.81 &             95.95 &             95.72 &         96.84 &           96.55 \\

\multicolumn{7}{r}{\footnotesize(Continued next page)}
\bottomrule
\end{tabular}
} % font size
\end{center}
\end{table*}

\begin{table*}[htp]
\label{fig:rocket_results}
\begin{center}
{\footnotesize
\begin{tabular}{lcccccc}

\toprule
Dataset &  rocket &  rocket\_noise\_1.0 &  rocket\_noise\_3.0 &  rocket\_noise\_5.0 &  rocket\_smote &  rocket\_timegan \\
\midrule
OSULeaf                        &   94.30 &             90.08 &             90.74 &             90.83 &         93.88 &           91.65 \\
OliveOil                       &   92.00 &             84.67 &             86.67 &             86.67 &         94.00 &           90.00 \\
PEMS-SF                        &   82.43 &             83.93 &             82.66 &             83.35 &         83.35 &           82.31 \\
PLAID                          &   23.99 &             26.29 &             27.41 &             27.82 &         14.15 &           35.42 \\
PenDigits                      &   97.87 &             97.77 &             97.75 &             97.71 &         97.72 &           97.66 \\
PhalangesOutlinesCorrect       &   83.38 &             82.45 &             82.26 &             82.52 &         82.70 &           83.24 \\
Plane                          &  100.00 &            100.00 &            100.00 &            100.00 &        100.00 &          100.00 \\
ProximalPhalanxOutlineAgeGroup &   85.46 &             85.17 &             85.56 &             85.27 &         84.10 &           85.07 \\
ProximalPhalanxOutlineCorrect  &   90.38 &             88.38 &             87.84 &             88.45 &         91.75 &           89.83 \\
ProximalPhalanxTW              &   81.46 &             77.56 &             77.46 &             77.56 &         76.98 &           80.29 \\
RacketSports                   &   90.66 &             90.92 &             91.05 &             90.53 &         91.32 &           91.58 \\
SelfRegulationSCP1             &   85.39 &             84.85 &             85.19 &             85.19 &         84.51 &           84.98 \\
SonyAIBORobotSurface1          &   92.18 &             91.95 &             91.75 &             91.38 &         93.71 &           91.61 \\
SonyAIBORobotSurface2          &   91.31 &             88.94 &             88.88 &             88.94 &         89.74 &           86.53 \\
SpokenArabicDigits             &   96.20 &             98.34 &             98.23 &             98.26 &         96.44 &           98.40 \\
StarLightCurves                &   98.06 &             98.11 &             97.98 &             97.83 &         97.81 &           98.13 \\
Strawberry                     &   98.11 &             97.41 &             97.30 &             97.41 &         98.11 &           98.11 \\
SwedishLeaf                    &   96.64 &             95.78 &             96.00 &             96.38 &         96.61 &           96.64 \\
Symbols                        &   97.41 &             97.89 &             97.45 &             97.03 &         97.57 &           97.81 \\
Trace                          &  100.00 &            100.00 &            100.00 &            100.00 &        100.00 &          100.00 \\
TwoLeadECG                     &   99.91 &             99.91 &             99.91 &             99.91 &         99.91 &           99.91 \\
TwoPatterns                    &  100.00 &            100.00 &            100.00 &            100.00 &        100.00 &          100.00 \\
UWaveGestureLibraryAll         &   97.59 &             97.44 &             97.45 &             97.43 &         97.54 &           97.51 \\
UWaveGestureLibraryX           &   85.48 &             85.39 &             85.49 &             85.53 &         85.32 &           85.47 \\
UWaveGestureLibraryY           &   77.36 &             77.92 &             77.81 &             77.63 &         77.87 &           78.11 \\
UWaveGestureLibraryZ           &   79.21 &             79.25 &             79.03 &             79.12 &         79.35 &           79.11 \\
Wafer                          &   99.80 &             99.78 &             99.81 &             99.80 &         99.86 &           99.80 \\
Wine                           &   81.11 &             90.74 &             89.26 &             88.89 &         80.74 &           85.19 \\
WordSynonyms                   &   75.27 &             73.92 &             71.10 &             71.41 &         75.42 &           72.98 \\
Worms                          &   74.55 &             63.12 &             64.16 &             68.57 &         72.73 &           68.31 \\
WormsTwoClass                  &   79.22 &             79.48 &             78.18 &             77.92 &         78.44 &           77.92 \\
Yoga                           &   91.07 &             90.67 &             90.85 &             90.89 &         90.86 &           91.11 \\
\bottomrule
\end{tabular}
} % font size
\end{center}
\end{table*}

\begin{table*}[htb]

\caption{Accuracy for InT baseline model on balanced datasets of the UCR/UEA archive \tr{add 5 scatter plots graph with a diagonal line (everything above diagonal means that augmentation wins)}\ro{scatter plot added in the main content of the paper, now remove this table?}}
\label{int_results}
\begin{center}
{\footnotesize
\begin{tabular}{lcccccc}
\toprule
Dataset &  InT &  InT\_noise\_1.0 &  InT\_noise\_3.0 &  InT\_noise\_5.0 &  InT\_smote &  InT\_timegan \\
\midrule
Adiac                          &   78.06 &          67.72 &          66.85 &          68.24 &      81.18 &        78.72 \\
CBF                            &   99.78 &          99.98 &          99.73 &          99.84 &      99.96 &        99.89 \\
Car                            &   84.33 &          88.00 &          86.67 &          84.67 &      90.33 &        86.67 \\
CharacterTrajectories          &   99.51 &          99.51 &          99.30 &          99.20 &      99.55 &        99.41 \\
ChlorineConcentration          &   86.99 &          85.35 &          84.10 &          85.20 &      86.58 &        78.24 \\
CinCECGTorso                   &   76.51 &          67.35 &          65.62 &          68.96 &      78.87 &        69.19 \\
CricketX                       &   85.18 &          82.56 &          83.03 &          83.18 &      84.87 &        83.90 \\
CricketY                       &   84.67 &          81.44 &          82.21 &          82.15 &      85.33 &        83.23 \\
CricketZ                       &   85.90 &          82.21 &          81.79 &          82.97 &      85.33 &        82.62 \\
DistalPhalanxOutlineAgeGroup   &   71.94 &          73.09 &          72.37 &          73.38 &      71.80 &        73.09 \\
DistalPhalanxOutlineCorrect    &   76.16 &          73.41 &          76.01 &          75.51 &      75.43 &        76.52 \\
DistalPhalanxTW                &   68.20 &          67.63 &          67.19 &          68.06 &      66.47 &        67.05 \\
DodgerLoopDay                  &   54.75 &          56.50 &          53.50 &          60.50 &      55.25 &        57.00 \\
ECG200                         &   87.00 &          90.20 &          92.20 &          90.60 &      91.40 &        90.40 \\
ECG5000                        &   93.36 &          93.48 &          93.43 &          93.47 &      94.27 &        93.75 \\
ECGFiveDays                    &  100.00 &         100.00 &         100.00 &          99.98 &     100.00 &       100.00 \\
EOGHorizontalSignal            &   57.96 &          57.02 &          54.81 &          54.20 &      57.46 &        55.41 \\
EOGVerticalSignal              &   47.24 &          47.93 &          46.96 &          47.51 &      46.91 &        45.91 \\
Earthquakes                    &   74.39 &          75.11 &          73.96 &          73.96 &      74.68 &        74.39 \\
EigenWorms                     &   92.37 &          92.62 &          89.31 &          89.57 &      94.66 &        86.77 \\
ElectricDevices                &   71.96 &          70.09 &          70.32 &          70.92 &      71.13 &        71.94 \\
Epilepsy                       &   97.10 &          97.39 &          96.81 &          96.96 &      97.25 &        96.96 \\
EthanolConcentration           &   23.19 &          24.33 &          20.15 &          22.81 &      24.52 &        23.57 \\
FaceFour                       &   95.00 &          95.45 &          92.05 &          93.41 &      94.32 &        94.32 \\
FacesUCR                       &   96.36 &          95.67 &          96.02 &          95.98 &      96.76 &        95.46 \\
FingerMovements                &   53.20 &          50.40 &          48.60 &          47.80 &      51.00 &        48.40 \\
Fish                           &   98.86 &          98.29 &          98.17 &          98.17 &      98.63 &        99.09 \\
FordA                          &   95.77 &          95.79 &          95.59 &          95.79 &      95.30 &        95.55 \\
FordB                          &   85.04 &          84.86 &          84.67 &          85.11 &      84.91 &        84.72 \\
GesturePebbleZ1                &   74.13 &          73.02 &          74.19 &          76.74 &      29.30 &        76.98 \\
GesturePebbleZ2                &   61.14 &          58.10 &          61.52 &          59.37 &      61.65 &        64.05 \\
GunPoint                       &   99.47 &          99.33 &          99.67 &          99.00 &     100.00 &        99.87 \\
GunPointAgeSpan                &   98.86 &          98.92 &          98.80 &          98.92 &      99.11 &        98.86 \\
GunPointMaleVersusFemale       &   99.68 &          99.37 &          99.37 &          99.43 &      99.43 &        99.30 \\
GunPointOldVersusYoung         &   95.43 &          96.06 &          95.49 &          96.19 &      95.62 &        96.89 \\
Ham                            &   72.95 &          72.00 &          71.43 &          72.19 &      71.24 &        73.71 \\
HandOutlines                   &   96.22 &          64.05 &          64.05 &          64.54 &      95.78 &        64.05 \\
Handwriting                    &   64.33 &          60.78 &          58.52 &          58.19 &      63.29 &        57.84 \\
Haptics                        &   51.75 &          50.65 &          43.83 &          44.16 &      51.36 &        50.19 \\
Heartbeat                      &   71.22 &          71.41 &          73.37 &          72.78 &      71.51 &        70.15 \\
Herring                        &   67.81 &          60.00 &          60.94 &          59.38 &      65.62 &        66.25 \\
InlineSkate                    &   30.40 &          31.09 &          22.80 &          23.64 &      37.60 &        30.04 \\
InsectEPGRegularTrain          &   99.68 &         100.00 &          99.76 &          99.52 &      99.92 &        99.52 \\
InsectEPGSmallTrain            &   95.58 &          95.42 &          95.66 &          94.78 &      95.10 &        94.62 \\
ItalyPowerDemand               &   96.58 &          96.56 &          96.91 &          96.56 &      96.64 &        96.72 \\
LSST                           &   69.40 &          65.25 &          62.40 &          62.04 &      67.60 &        69.91 \\
Lightning2                     &   82.62 &          86.56 &          88.52 &          87.87 &      85.57 &        85.57 \\
Lightning7                     &   80.55 &          75.62 &          77.40 &          76.71 &      78.63 &        77.81 \\
Mallat                         &   92.49 &          95.08 &          93.37 &          91.28 &      95.38 &        92.54 \\
MedicalImages                  &   77.74 &          75.21 &          74.11 &          74.11 &      77.37 &        76.24 \\
MelbournePedestrian            &   90.79 &          90.54 &          90.77 &          91.06 &      90.88 &        90.81 \\
MiddlePhalanxOutlineAgeGroup   &   55.45 &          51.82 &          51.56 &          55.32 &      50.52 &        55.97 \\
MiddlePhalanxOutlineCorrect    &   81.24 &          82.47 &          81.58 &          81.27 &      81.37 &        81.10 \\
MiddlePhalanxTW                &   54.03 &          54.81 &          56.49 &          55.45 &      52.21 &        48.83 \\
NonInvasiveFetalECGThorax1     &   93.14 &          89.97 &          91.36 &          90.99 &      92.87 &        90.35 \\
NonInvasiveFetalECGThorax2     &   93.39 &          91.95 &          92.83 &          92.88 &      93.73 &        92.20 \\

\multicolumn{7}{r}{\footnotesize(Continued next page)}
\bottomrule
\end{tabular}
} % font size
\end{center}
\end{table*}

\begin{table*}[htp]
\label{fig:rocket_results}
\begin{center}
{\footnotesize
\begin{tabular}{lcccccc}
\toprule
Dataset &  InT &  InT\_noise\_1.0 &  InT\_noise\_3.0 &  InT\_noise\_5.0 &  InT\_smote &  InT\_timegan  \\
\midrule
OSULeaf                        &   94.55 &          91.24 &          89.75 &          90.91 &      94.88 &        89.42 \\
OliveOil                       &   40.00 &          40.00 &          40.00 &          40.00 &      40.00 &        40.00 \\
PEMS-SF                        &   81.21 &          78.61 &          77.75 &          78.61 &      78.61 &        78.61 \\
PLAID                          &   68.90 &          55.49 &          54.38 &          54.97 &      67.37 &        62.76 \\
PenDigits                      &   98.96 &          98.74 &          98.77 &          98.99 &      98.99 &        98.79 \\
PhalangesOutlinesCorrect       &   83.80 &          83.82 &          83.57 &          83.40 &      82.47 &        82.91 \\
Plane                          &  100.00 &         100.00 &         100.00 &         100.00 &     100.00 &       100.00 \\
ProximalPhalanxOutlineAgeGroup &   85.66 &          84.49 &          85.46 &          84.00 &      85.76 &        85.46 \\
ProximalPhalanxOutlineCorrect  &   91.07 &          91.89 &          91.75 &          91.96 &      91.62 &        92.16 \\
ProximalPhalanxTW              &   79.12 &          78.54 &          81.37 &          81.85 &      77.95 &        79.02 \\
RacketSports                   &   87.89 &          89.80 &          89.80 &          87.83 &      88.03 &        88.82 \\
SelfRegulationSCP1             &   76.18 &          74.74 &          76.25 &          76.25 &      77.27 &        77.00 \\
SonyAIBORobotSurface1          &   89.78 &          91.91 &          90.72 &          89.08 &      88.99 &        87.49 \\
SonyAIBORobotSurface2          &   95.74 &          94.00 &          95.17 &          95.74 &      95.57 &        91.29 \\
SpokenArabicDigits             &   99.14 &          98.93 &          98.79 &          99.41 &      98.93 &        98.98 \\
StarLightCurves                &   97.92 &          97.34 &          97.28 &          97.32 &      97.76 &        97.27 \\
Strawberry                     &   97.78 &          97.41 &          97.24 &          97.46 &      97.95 &        97.78 \\
SwedishLeaf                    &   96.10 &          94.62 &          95.17 &          95.12 &      96.00 &        95.90 \\
Symbols                        &   97.57 &          98.17 &          97.97 &          97.49 &      97.83 &        97.69 \\
Trace                          &  100.00 &         100.00 &         100.00 &         100.00 &     100.00 &       100.00 \\
TwoLeadECG                     &   99.70 &          99.26 &          99.84 &          99.91 &      99.81 &        99.81 \\
TwoPatterns                    &  100.00 &         100.00 &         100.00 &         100.00 &     100.00 &       100.00 \\
UWaveGestureLibraryAll         &   92.98 &          92.65 &          91.94 &          92.66 &      93.19 &        92.03 \\
UWaveGestureLibraryX           &   81.70 &          81.02 &          81.99 &          80.33 &      81.53 &        81.36 \\
UWaveGestureLibraryY           &   76.79 &          73.29 &          74.68 &          72.80 &      76.51 &        74.86 \\
UWaveGestureLibraryZ           &   75.70 &          75.87 &          74.44 &          75.64 &      74.43 &        74.94 \\
Wafer                          &   99.81 &          99.85 &          99.83 &          99.83 &      99.88 &        99.89 \\
Wine                           &   50.00 &          48.15 &          50.00 &          50.00 &      50.00 &        55.19 \\
WordSynonyms                   &   71.35 &          66.39 &          59.44 &          54.61 &      71.47 &        59.06 \\
Worms                          &   80.26 &          77.06 &          78.79 &          75.32 &      81.30 &        77.40 \\
WormsTwoClass                  &   73.51 &          77.06 &          71.86 &          76.19 &      74.29 &        75.32 \\
Yoga                           &   90.67 &          89.01 &          89.55 &          89.45 &      90.12 &        89.45 \\
\bottomrule
\end{tabular}
} % font size
\end{center}
\end{table*}
